# Supplementary material for: Resonance control of graphene drum resonator in nonlinear regime by standing wave of light
Source: arXiv:1705.05056 source file (2017-05-15)
Supplement: Supplementary file 1 [file inoue_Supp.pdf]

*Supplementary information*

# Resonance control of graphene drum resonator in nonlinear regime by standing wave of light

Taichi Inoue, Yuki Anno, Yuki Imakita, Kuniharu Takei, Takayuki Arie, and Seiji Akita[1]

Department of Physics and Electronics, Osaka Prefecture University, Sakai 599-8531, Japan

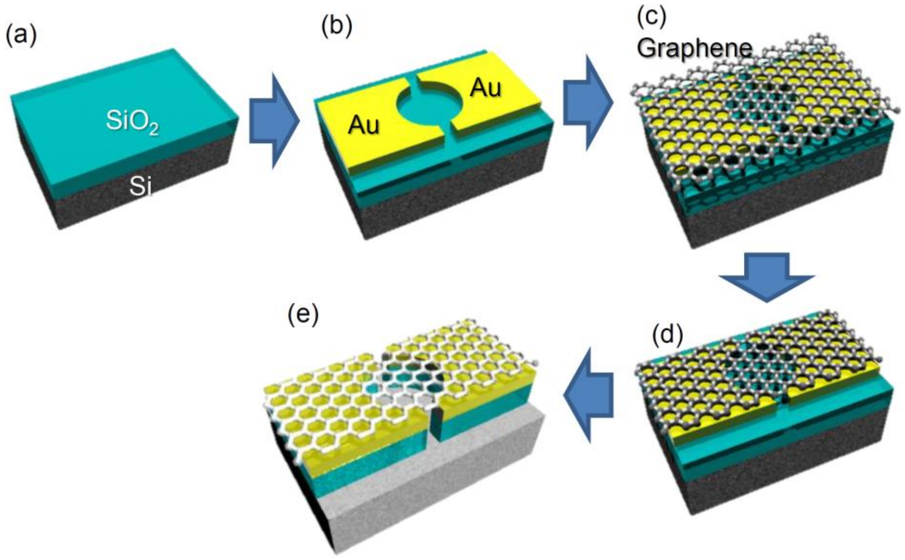


**Fig. S1 Schematic illustration of the flow of device fabrication.** (a) Si substrate with 300 nm – thick $SiO_2$. (b) Au electrodes fabricated by conventional photolithography. (c) Transfer CVD-grown graphene. (d) Trimming of graphene by plasma etching. (e) Etching of $SiO_2$ layer underneath graphene.

[1] e-mail: akita@pe.osakafu-u.ac.jp

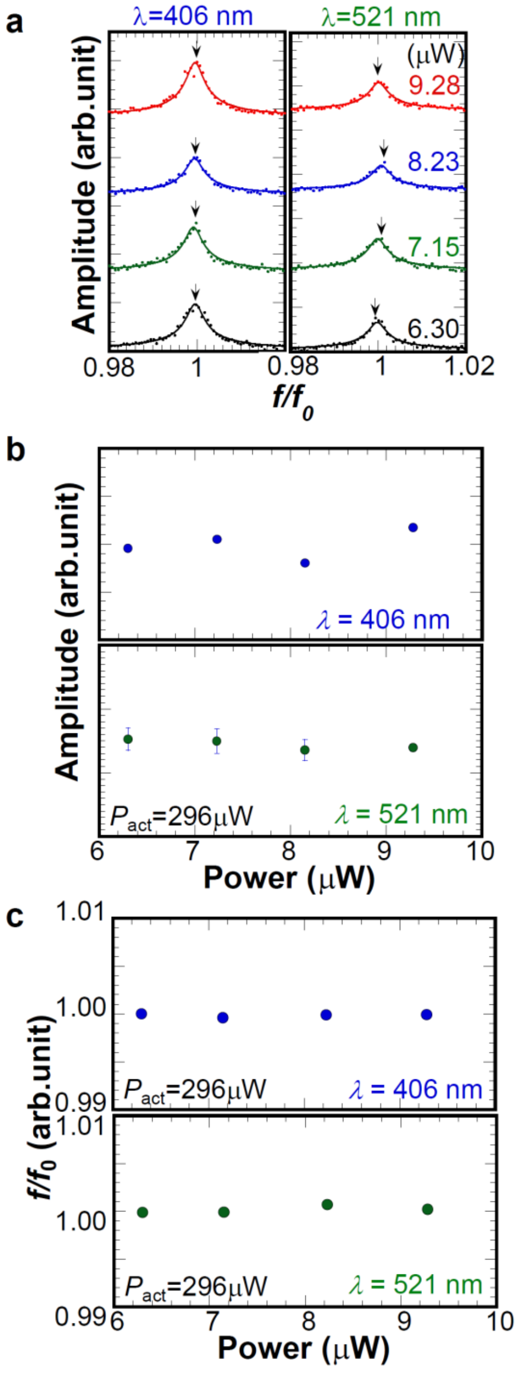


**Fig. S2 Resonance properties of G-MR under linear oscillation regime.** (a) Resonance curves measured under various probe laser intensity with the different wavelengths of 406 and 521 nm. Solid lines for respective measured response are the fitting curves fitted by the same Q factor of 250. (b) and (c) are probe laser power dependences of the oscillation amplitude and $f/f_0$, respectively.
